# Supplementary material for: The Anatomy of Electro-Weak Symmetry Breaking. I: The Higgs boson in the Standard Model
Source: arXiv:hep-ph/0503172 source file (2005-05-03)
Supplement: Supplementary file 1 [file hsm4-refs.tex]

%%%%%%%%%%%%%%%%%%%%%% Section 4.1: Introduction %%%%%%%%%%% 

\bibitem{TESLAtdr} J. Andruszkow et al, TESLA Technical Design Report, Part II,
{\it The Accelerator}, DESY 2001-011, ECFA 2001-209

\bibitem{NLCtdr} {\it Zeroth Order Design Report for the Next Linear Collider},
SLAC Report 474, 1996; {\it 2001 Report on the Next Linear Collider},
Fermilab-Conf-01-075-E. 

\bibitem{JLCtdr} KEK-Report 97-1, 1997.

\bibitem{CLICtdr} R.W.~Assmann et al.,``{\it A 3-TeV $\ee$  linear collider 
based on CLIC technology}", CERN-2000-008.

\bibitem{eeReviews} Selected reviews for machine and detector physics. 

\bibitem{TESLA} J.A. Aguilar-Saavedra et al, TESLA Technical Design Report, 
Part III, {\it Physics at an $e^+e^-$ Linear Collider}, hep-ph/0106315.

\bibitem{NLC} T. Abe et al, {\it Linear Collider Physics Resource Book for 
Snowmass 2001}, hep-ex/0106055-58.

\bibitem{JLC} K. Abe et al, {\it Particle Physics Experiments at JLC},
hep-ph/0109166.

\bibitem{CLIC} CLIC Report. 

\bibitem{gamma-machine} I.~Ginzburg, G.~Kotkin, V.~Serbo and V.~Telnov, 
Pizma ZhETF 34 (1981) 514 and JETP Lett. 34 (1982) 491;
I.~Ginzburg, G.~Kotkin, V.~Serbo and V.~Telnov, Nucl.  Instr. \& Meth. 
205 (1983) 47.

\bibitem{gamma-machine2} I.~Ginzburg, G.~Kotkin, S.~Panfil, V.~Serbo and 
V.~Telnov, Nucl. Instr. Meth. 219 (1984) 5.
\bibitem{gammaReview} Review on gamma-machines. 
\bibitem{muonReview} Review on muons colliders. 

%%%%%%%%%%%%%%%%%%%%%%%%%Section 4.2 %%%%%%%%%%%%%%%%%%%%%%%%%%%%%%%%%%%%%
\bibitem{EGN} 
J. Ellis, M.K. Gaillard, and D.V. Nanopoulos, Nucl. Phys.  B106 (1976) 292.
\bibitem{LQT}
B.W. Lee, C. Quigg and H.B. Thacker, Phys. Rev. D16 (1977) 1519.
\bibitem{Bjorken-process} 
J.D. Bjorken, Proc. 1976 SLAC Summer Inst. Part. 
Phys., ed. M.C. Zipf (SLAC report 198,1977) 1. 
\bibitem{Higgs-strahlung}
B.L. Joffe and V.A. Khoze, Sov. J. Part. Phys. {\bf 9} (1978) 50; 
D.R.T. Jones and S.T. Petcov, Phys. Lett. B84 (1979) 440; 
F.A. Behrends and R. Kleiss, Nucl. Phys. B260 (1985) 32.
\bibitem{Wfus1}
R.N.\ Cahn and S.\ Dawson, Phys.\ Lett.\ B136 (1984) 196; 
K.\ Hikasa, Phys.\ Lett.\ B164 (1985) 341. 

\bibitem{Wfus2}
G.\ Altarelli, B.\ Mele and F.\ Pitolli, Nucl.\ Phys.\ B287 (1987) 205.

\bibitem{Wfus3} W. Kilian, M. Kr\"amer and P.M. Zerwas, Phys. Lett. B373 
(1996) 135.
\bibitem{ttH1} Old ttH
\bibitem{ttH2} Our ttH. 
\bibitem{HHZ1} Old HHZ, Haber et al. 
\bibitem{HHW1} Old HHW
\bibitem{DKMZ} Maggies paper.
\bibitem{Hgamma1} Old Hgamma.
\bibitem{Hgamma2} Our Hgamma.
\bibitem{HHloop1} Old HH from loop.
\bibitem{HHloop2} Our HH from loop. 
\bibitem{HVVprod} HVV production.
\bibitem{Hffprod} Hff production.
\bibitem{HppP1}
\bibitem{HppP2}
\bibitem{HppP3}
\bibitem{egammaP}
\bibitem{mumuP1}
\bibitem{mumuP2}
\bibitem{RCHZ} 
J. Fleischer and F. Jegerlehner, Nucl. Phys. B216 (1983) 469;
B. A. Kniehl, Z. Phys. C55 (92) 605;
A. Denner, J. K\"ublbeck, R. Mertig and M. B\"ohm, Z. Phys. C56 (92) 261.
\bibitem{RCWW1} 
A. Denner, S. Dittmaier, M. Roth and M. M. Weber, Nucl. Phys. B660 (2003) 289.

\bibitem{RCWW2} 
G. B\'elanger, F. Boudjema, J. Fujimoto, T. Ishikawa, T. Kaneko, 
K. Kato and Y. Shimizu, Phys. Lett. B559 (2003) 252. 

\bibitem{RCWW3} F. Jegerlehner and O. Tarasov, Nucl. Phys. Proc. Suppl. 116 
(2003) 83.  

\bibitem{RCZZ} F. Boudjema, J. Fujimoto, T. Ishikawa, T. Kaneko, K. Kato
Y. Kurihara, Y. Shimizu, S. Yamashita, Y. Yasui, hep-ph/0404098. 

\bibitem{RCTTqcd1} S. Dittmaier, M. Kr\"amer, Y. Liao, M. Spira and P.M. Zerwas,
Phys. Lett. B441 (1998) 383. 

\bibitem{RCTTqcd2} S. Zhu, hep-ph/0212273;  for the correction to the dominant
channel see also S. Dawson and L. Reina,  Phys. Rev. D59 (1999) 054012.

\bibitem{RCTTew1} G. B\'elanger, F. Boudjema, J. Fujimoto, T. Ishikawa, 
T. Kaneko, K. Kato, Y. Shimizu and Y. Yasui, Phys. Lett. B571 (2003) 163; 

\bibitem{RCTTew2}
A. Denner, S. Dittmaier, M. Roth and  M.M. Weber, Phys. Lett. B575 (2003) 290.

\bibitem{RCTTew0}
You Yu, Ma Wen-Gan, Chen Hui, Zhang Ren-You, Sun Yan-Bin and Hou Hong-Sheng,
Phys. Lett. B571 (2003) 85.

\bibitem{RCZHH}  G. B\'elanger, F. Boudjema, J. Fujimoto, T. Ishikawa, 
T. Kaneko, Y. Kurihara, K. Kato and Y. Shimizu, Phys. Lett. B576 (2003) 152;
Zhang Ren-You, Ma Wen-Gan, Chen Hui, Sun Yan-Bin and Hou Hong-Sheng,
Phys. Lett. B578 (2004) 349.

%%%%%%%%%%%%%%%%%%%%%%%%%%%%%%%%%%%%%%%%%%%%%%%%%%%%%%%%%%%%%%%%%%%%%%%%%%%%
\bibitem{High-Precision} The LEP Collaborations (ALEPH, DELPHI, L3 and OPAL), 
the LEP Electroweak Working Group and the SLD Heavy Flavour Group, {\it A
combination of preliminary Electroweak measurements and constraints on the
Standard Model}, hep-ex/0312O23; {\tt http://lepewwg.web.cern.ch/LEPEWWG};
for an update see, G. Altarelli and M. Grunewald, hep-ph/0404165.
\bibitem{MW-Tevatron} The CDF and D0 collaborations, hep-ex/0311039.
\bibitem{Mt-Tevatron} The CDF and D0 collaborations and the Tevatron 
Electroweak Working Group, hep-ex/0404010.
\bibitem{alphas-review} G. Altarelli, hep-ph/0204179;
S. Bethke, Nucl. Phys. Proc.Suppl. 121 (2003) 74 [hep-ex/0211012];
I. Hinchliffe in Ref.~\cite{PDG}.
\bibitem{PDG} Particle Data Group, K. Hagiwara et al., Phys. Rev. D66 
(2002) 010001.
\bibitem{Z-Physics} {\it Z Physics at LEP1}, CERN Report 89--08 (1989),
eds. G. Altarelli, R. Kleiss and C. Verzegnassi; see this reference for 
earlier work. 
\bibitem{W-Physics} {\it Physics at LEP2}, CERN Report 96--01, eds. G. 
Altarelli, T. Sj\"ostrand and F. Zwirner.  
\bibitem{Bjorken-process} 
J.D. Bjorken, Proc. 1976 SLAC Summer Inst. Part. 
Phys., ed. M.C. Zipf (SLAC report 198,1977) 1. 
\bibitem{Z-h-gamma1} R.N. Cahn, M.S. Chanowitz and N. Fleishon, Phys. Lett.
82B (1979) 113. 
\bibitem{Z-h-gamma2} L. Bergstrom and G. Hulth, Nucl. Phys. B259 (1985) 137.
\bibitem{EGN} 
J. Ellis, M.K. Gaillard, and D.V. Nanopoulos, Nucl. Phys.  B106 (1976) 292.
\bibitem{LQT}
B.W. Lee, C. Quigg and H.B. Thacker, Phys. Rev. D16 (1977) 1519.
\bibitem{Higgs-strahlung}
B.L. Joffe and V.A. Khoze, Sov. J. Part. Phys. {\bf 9} (1978) 50; 
D.R.T. Jones and S.T. Petcov, Phys. Lett. B84 (1979) 440; 
F.A. Behrends and R. Kleiss, Nucl. Phys. B260 (1985) 32.
\bibitem{LEP2-Higgs-Th} M. Carena, Peter M. Zerwas (conv.) et al., 
{\it Higgs Physics at LEP2} in \cite{W-Physics}, 
Part I, p. 351 [hep-ph/9602250]. 
\bibitem{LEP2-Higgs-exp} The LEP Collaboration (ALEPH, DELPHI, L3 and OPAL), 
Phys. Lett. B565 (2003) 61 [hep-ex/0306033]. 
\bibitem{LEP2-Higgs-ind} The LEP Collaboration (ALEPH, DELPHI, L3 and OPAL), 
hep-ex/0107032 (invisible decays) and hep-ex/0107034 (flavor blind hadronic 
decays).
